# Supplementary material for: Energy flux enhancement, intermittency and turbulence via Fourier triad phase dynamics in 1D Burgers equation
Source: arXiv:1705.08960 ancillary file (2018-05-25)
Supplement: Supplementary file 1 [file Ancillary_Material_arXiv_Final.pdf]

# Energy flux enhancement, intermittency and turbulence via Fourier triad phase dynamics in 1D Burgers equation: SUPPLEMENTARY MATERIAL

**Brendan P. Murray and Miguel D. Bustamante†**

Institute for Discovery, Department of Mathematics and Statistics, University College Dublin, Belfield D4, Ireland

(Received xx; revised xx; accepted xx)

Find below table of the power law fit values for the real-space multi-point correlation functions (structure functions) statistics defined in equation (1.8) in the main text. Values are given for both the full PDE (Partial Differential Equation) and phase-only models. In each case three sets of results are presented. The first is for statistics over all time ($R \in [0, 1]$), the second for time when we have a high level of triad phase synchronisation defined similarly to the main text as time when $R > 0.95$. The final data is for when the triad phases are not synchronised, defined as the complement ad the second case ($R \leqslant 0.95$). Fitted values are presented for both structure functions $S^p(r)$ and $S^p_{\rm abs}(r)$.

Also included are figures 1 and 2 which show the $S^p(r)$ and $S^p_{\rm abs}(r)$ as a function of $r$ and the range (highlighted region) where the fit values were calculated. Also included as insets are the local slope values. Figure 1 shows the results for the full PDE model with figure 2 showing the same analysis repeated for the phase-only model.

Finally, we provide the following links to YouTube videos showing simulation results from:

- Full-PDE 1D Burgers numerical simulation with stochastic forcing:

`www.youtube.com/watch?v=xOSokgDxmcU`

- Phase-only 1D Burgers numerical simulation with stochastic forcing:

`www.youtube.com/watch?v=OOY5Chd6SrE`

Snapshots and descriptions of these videos are provided in figures 3 and 4 below.

† Email address for correspondence: miguel.bustamante@ucd.ie

| | **Full PDE** | | | | | | **Phase-only Model** | | | | | |
|---|---|---|---|---|---|---|---|---|---|---|---|---|
| | $R \in [0,1]$ | | $R \leqslant 0.95$ | | $R > 0.95$ | | $R \in [0,1]$ | | $R \leqslant 0.95$ | | $R > 0.95$ | |
| $p$ | $\zeta^p$ | $\zeta^p_{\text{abs}}$ | $\zeta^p$ | $\zeta^p_{\text{abs}}$ | $\zeta^p$ | $\zeta^p_{\text{abs}}$ | $\zeta^p$ | $\zeta^p_{\text{abs}}$ | $\zeta^p$ | $\zeta^p_{\text{abs}}$ | $\zeta^p$ | $\zeta^p_{\text{abs}}$ |
| 1 | - | 0.994 | - | 0.993 | - | 0.995 | - | 0.614 | - | 0.496 | - | 0.974 |
| 2 | 1.027 | 1.027 | 1.037 | 1.037 | 1.020 | 1.020 | 1.037 | 1.037 | 1.037 | 1.037 | 1.037 | 1.037 |
| 3 | 1.007 | 1.008 | 1.017 | 1.019 | 1.002 | 1.003 | 1.071 | 1.081 | 1.236 | 1.247 | 1.007 | 1.010 |
| 4 | 1.007 | 1.007 | 1.022 | 1.022 | 1.002 | 1.002 | 1.074 | 1.074 | 1.268 | 1.268 | 1.011 | 1.011 |
| 5 | 1.006 | 1.006 | 1.029 | 1.029 | 1.002 | 1.002 | 1.073 | 1.074 | 1.283 | 1.285 | 1.014 | 1.014 |
| 6 | 1.006 | 1.006 | 1.038 | 1.038 | 1.001 | 1.001 | 1.076 | 1.076 | 1.307 | 1.307 | 1.018 | 1.018 |

TABLE 1. Fitted values of power-law indices $\zeta^p$ and $\zeta^p_{\text{abs}}$ for the multi-point correlation functions (structure functions) $S^p(r)$ and $S^p_{\text{abs}}(r)$ in both the Full PDE and Phase-Only Models. Fit was conducted over the range $0.008 \leqslant r \leqslant 0.063$ which corresponds to our chosen inertial range of $100 \leqslant k \leqslant 750$. Region of fit corresponds to the highlighted range in figures 1 and 2 with local slopes plots shown in the insets.

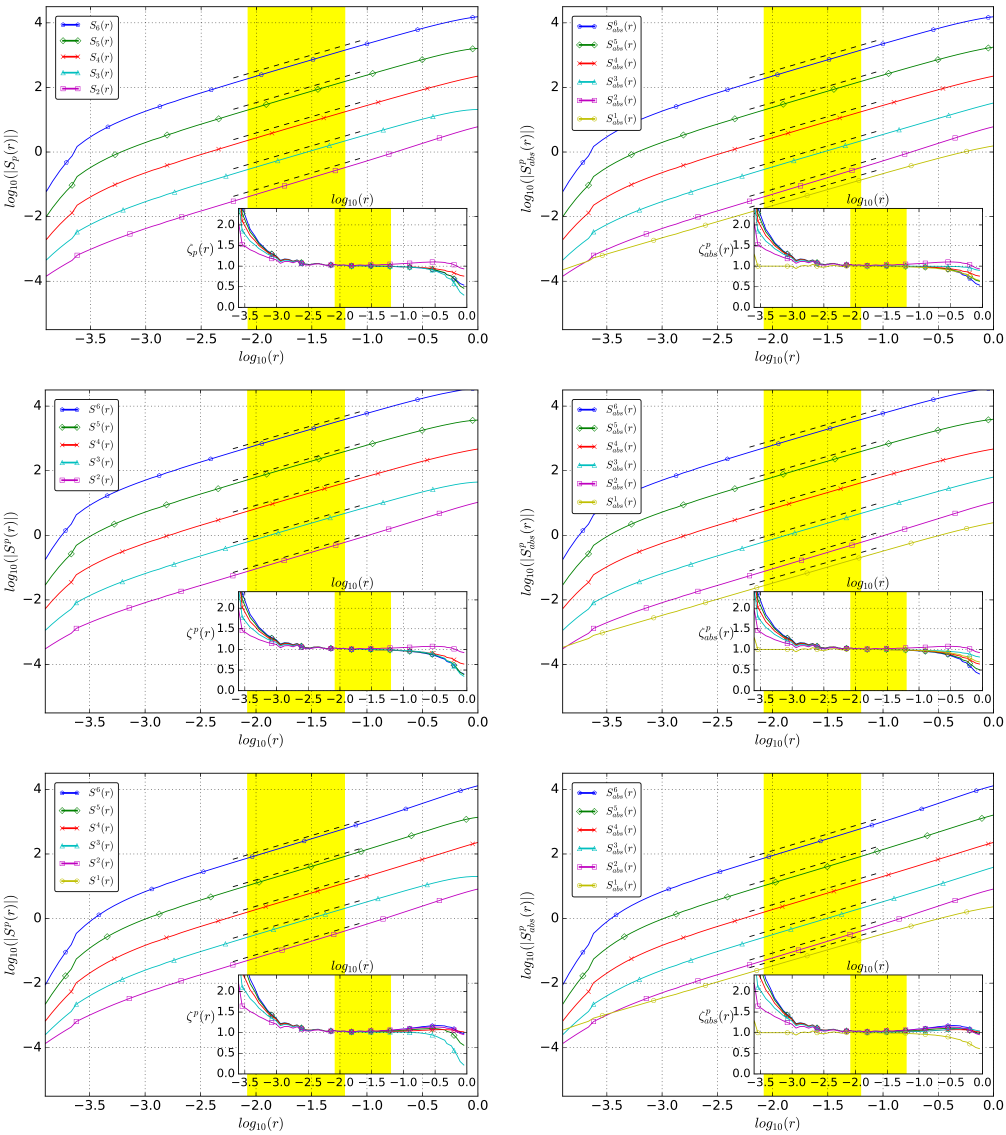


FIGURE 1. Multi-point correlation functions (structure functions) statistics over full statistically stationary state for the full PDE model. **Top Left**: Structure function $S^p(r)$ as a function of $r$ and (inset) the associated local slopes $\zeta^p(r)$. **Top Right**: Structure function $S^p_{\text{abs}}(r)$ as a function of $r$ and (inset) the associated local slopes $\zeta^p_{\text{abs}}(r)$. **Middle Left**: Conditional time ($R > 0.95$) structure function $S^p(r)$ as a function of $r$ and (inset) the associated local slopes $\zeta^p(r)$. **Middle Right**: Conditional time ($R > 0.95$) structure function $S^p_{\text{abs}}(r)$ as a function of $r$ and (inset) the associated local slopes $\zeta^p_{\text{abs}}(r)$. **Bottom Left**: Conditional time ($R \leqslant 0.95$) structure function $S^p(r)$ as a function of $r$ and (inset) the associated local slopes $\zeta^p(r)$. **Bottom Right**: Conditional time ($R \leqslant 0.95$) structure function $S^p_{\text{abs}}(r)$ as a function of $r$ and (inset) the associated local slopes $\zeta^p_{\text{abs}}(r)$.

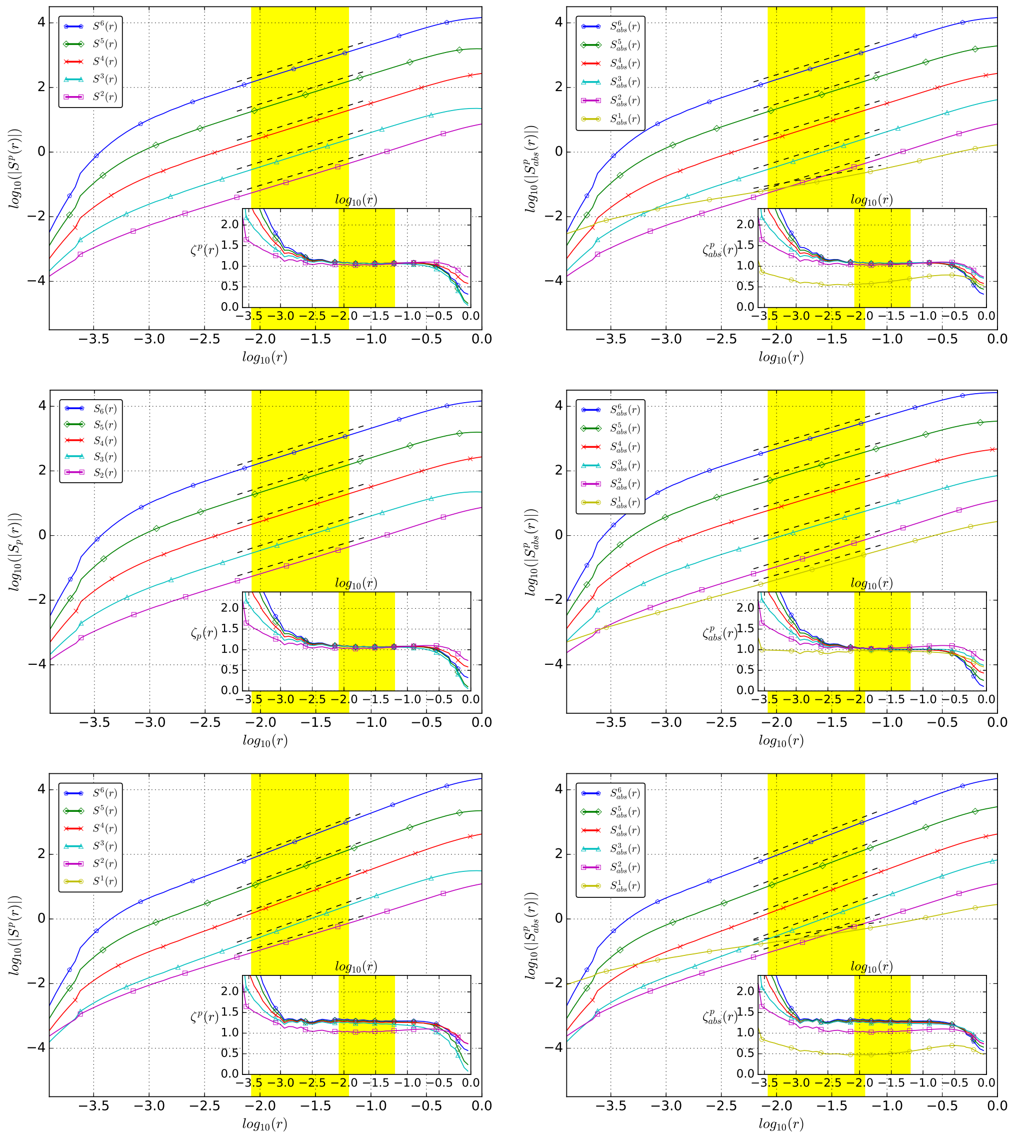


FIGURE 2. Multi-point correlation functions (structure functions) statistics over full statistically stationary state for the Phase-only PDE model. **Top Left**: Structure function $S^p(r)$ as a function of $r$ and (inset) the associated local slopes $\zeta^p(r)$. **Top Right**: Structure function $S^p_{\text{abs}}(r)$ as a function of $r$ and (inset) the associated local slopes $\zeta^p_{\text{abs}}(r)$. **Middle Left**: Conditional time ($R > 0.95$) structure function $S^p(r)$ as a function of $r$ and (inset) the associated local slopes $\zeta^p(r)$. **Middle Right**: Conditional time ($R > 0.95$) structure function $S^p_{\text{abs}}(r)$ as a function of $r$ and (inset) the associated local slopes $\zeta^p_{\text{abs}}(r)$. **Bottom Left**: Conditional time ($R \leqslant 0.95$) structure function $S^p(r)$ as a function of $r$ and (inset) the associated local slopes $\zeta^p(r)$. **Bottom Right**: Conditional time ($R \leqslant 0.95$) structure function $S^p_{\text{abs}}(r)$ as a function of $r$ and (inset) the associated local slopes $\zeta^p_{\text{abs}}(r)$.

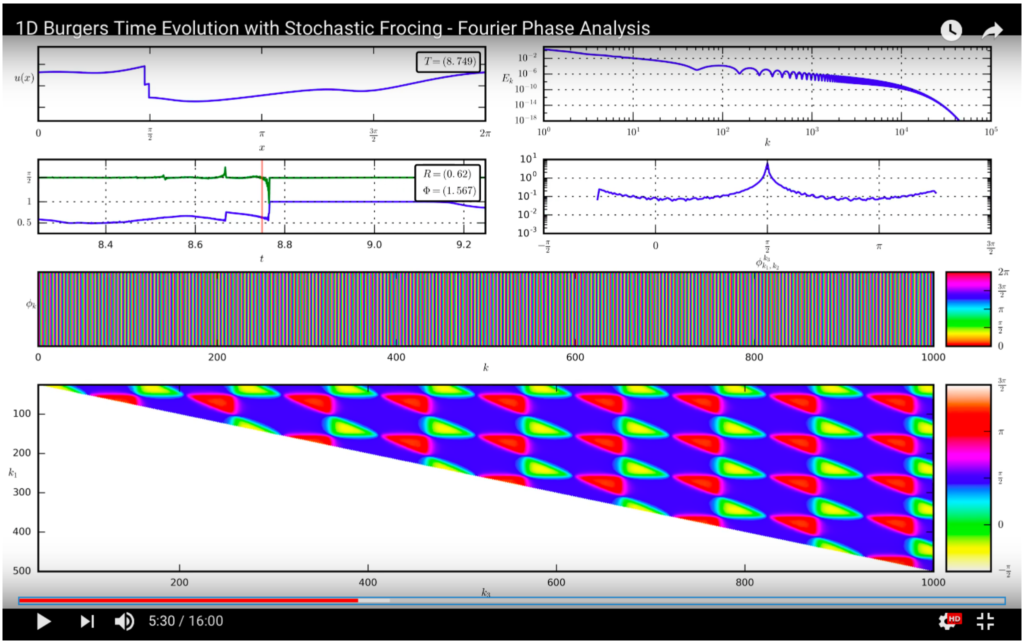


FIGURE 3. Snapshot of YouTube video (`www.youtube.com/watch?v=x0SokgDxmcU`) showing the results of a full-PDE 1D Burgers pseudo-spectral numerical simulation with stochastic forcing. Technical details as in Section 2 "Numerical Results for Large Scale Forcing" of main paper: $4^{\text{th}}$-order Adams-Bashforth time-stepping scheme, number of collocation points $N = 2^{18}$, largest resolved wavenumber $k_{\max} = N/3 \approx 87\,381$, time step $\delta t \sim 10^{-6}$. Forcing range: $k_f \in [1,3]$. Viscosity value $\nu = 2\times10^{-4}$, average total energy $\overline{E} \equiv \langle E(t)\rangle_t \approx 5.25$, average energy dissipation rate $\overline{\epsilon} \equiv \langle \epsilon(t)\rangle_t \approx 8.08$. Kolmogorov length and time microscales: $\eta \equiv (\nu^3/\overline{\epsilon})^{1/4} \approx 0.001$ and $\tau_\eta \equiv (\nu/\overline{\epsilon})^{1/2} \approx 0.005$. Reynolds number: $\mathrm{Re} \equiv ((2\pi/k_f)/\eta)^{4/3} \approx 2.7 \times 10^4$. **Top left panel:** time evolution of the real space solution $u(x,t)$ over the periodic spatial domain $x \in [0, 2\pi)$. **Top right panel:** time evolution of the Fourier energy spectrum $E_k$ as a function of the wavenumber $k$. **Second row, left panel:** sliding time window of the evolution of the triad phase order parameters $R$ and $\varPhi$ for triads composed of modes exclusively in the inertial range $k \in [50, 1000]$. **Second row, right panel:** time evolution of the PDF of the Fourier triad phases, also for the same set of triads in the inertial range. **Third row:** vertical striped bars coloured to show the values of the individual Fourier phases $\phi_k$ for $k \in [0, 1000]$ with $k$ on the horizontal axis. **Bottom panel:** time evolution of the Fourier triad phases $\varphi^{k_3}_{k_1,k_3-k_1}$ as a function of $(k_1, k_3)$, with $50 < k_1 < 500$ (vertical axis) and $50 < k_3 < 1000$ (horizontal axis). Due to symmetry, only half of the plot (upper triangle) is shown and the colour indicates the value of the Fourier triad phase.

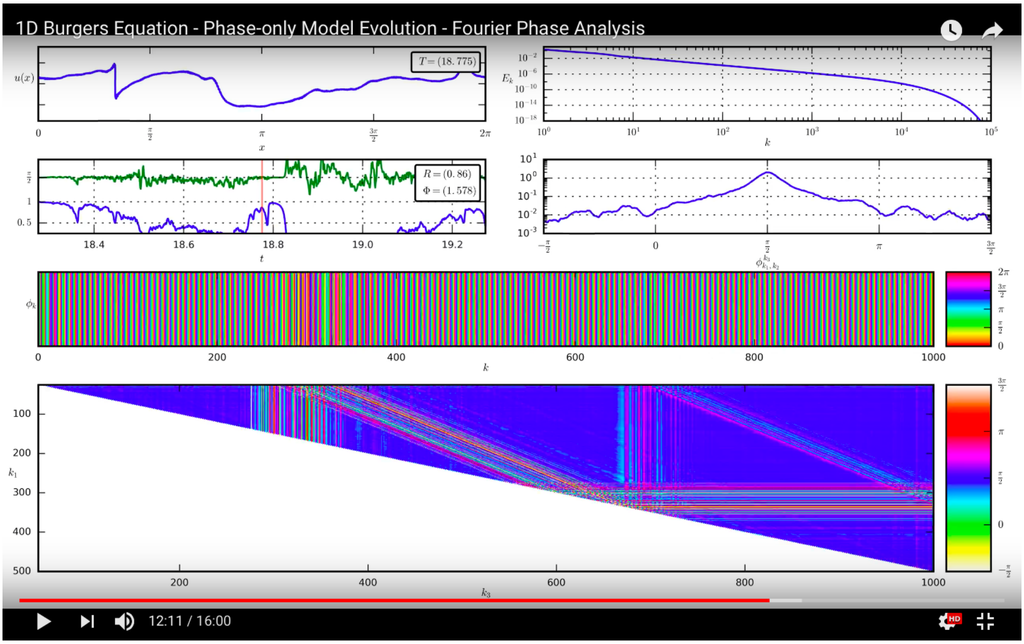


FIGURE 4. Snapshot of YouTube video (`www.youtube.com/watch?v=OOY5Chd6SrE`) showing the results of a phase-only 1D Burgers pseudo-spectral numerical simulation with stochastic forcing. Technical details as in Section 4 "Phase-Only Model" of main paper: 4$^{\text{th}}$-order Adams-Bashforth time-stepping scheme, number of collocation points $N = 2^{18}$, largest resolved wavenumber $k_{\max} = N/3 \approx 87\,381$, time step $\delta t \sim 10^{-6}$. Forcing range: $k_f \in [1, 3]$. Fourier energy spectrum is "frozen" in time and equal to the time-averaged energy spectrum obtained from a statistically-stationary full-PDE 1D Burgers simulation with stochastic forcing, with effective Reynolds number Re $\approx 2.7 \times 10^4$. **Top left panel:** time evolution of the real space solution $u(x,t)$ over the periodic spatial domain $x \in [0, 2\pi)$. **Top right panel:** "frozen" Fourier energy spectrum $E_k$ as a function of the wavenumber $k$. **Second row, left panel:** sliding time window of the evolution of the triad phase order parameters $R$ and $\Phi$ for triads composed of modes exclusively in the inertial range $k \in [50, 1000]$. **Second row, right panel:** time evolution of the PDF of the Fourier triad phases, also for the same set of triads in the inertial range. **Third row:** vertical striped bars coloured to show the values of the individual Fourier phases $\phi_k$ for $k \in [0, 1000]$ with $k$ on the horizontal axis. **Bottom panel:** time evolution of the Fourier triad phases $\varphi_{k_1, k_3 - k_1}^{k_3}$ as a function of $(k_1, k_3)$, with $50 < k_1 < 500$ (vertical axis) and $50 < k_3 < 1000$ (horizontal axis). Due to symmetry, only half of the plot (upper triangle) is shown and the colour indicates the value of the Fourier triad phase.
